# Supplementary material for: Ballistic thermophoresis of adsorbates on free-standing graphene
Source: arXiv:1708.06198 ancillary file (2017-08-21)
Supplement: Supplementary file 1 [file SI.pdf]

# Ballistic thermophoresis of adsorbates on free-standing graphene

**Supporting Information**

Emanuele Panizon[a], Roberto Guerra[a,b] and Erio Tosatti[a,c,d,1]

[a] *International School for Advanced Studies (SISSA), Via Bonomea 265, 34136 Trieste, Italy*
[b] *Dipartimento di Fisica, Università degli Studi di Milano, Via Celoria 16, 20133 Milano, Italy*
[c] *The Abdus Salam International Centre for Theoretical Physics (ICTP), Strada Costiera 11, 34151 Trieste, Italy*
[d] *CNR-IOM Democritos National Laboratory, Via Bonomea 265, 34136 Trieste, Italy*

## Cluster adsorption as a function of alignment

The static and dynamic properties of a gold cluster on graphene depend on the respective alignment.

The oscillations of the adhesion energy as a function of $\theta$, visible in Fig. S1, reflect a nanoscale remnant of the underlying moiré pattern connected with the incommensurability between the triangular Au(111) contact face and the honeycomb graphene lattice. In particular, the symmetric local minima at $\theta = \pm 9°$ are found by increasing cluster sizes (as shown here in Fig S1 for $Au_{1358}$) to get deeper and converge toward a smaller value, foreshadowing the emergence of a spontaneous Novaco-McTague misalignment [1, 2] for infinite contact size. For $Au_{459}$, the six fully aligned orientations $\theta =$ 0, $\pm 60°$, $\pm 120°$, 180 ° correspond to a pinned state, where the cluster has an energy barrier against both rotations and translations.

Since the rotational energy barrier is smaller than the translational one [3, 4], thermal rotations are the first to be excited upon heating. Their effect is to make the interface misaligned. In this "incommensurate" state the translational barrier drops dramatically, allowing positional diffusion to occur. The overall diffusive motion of the cluster consists therefore of an alternation of locked states at specific angles where only vibrations take place, and of diffusive states where the rotationally depinned cluster executes fast translations [3, 4].

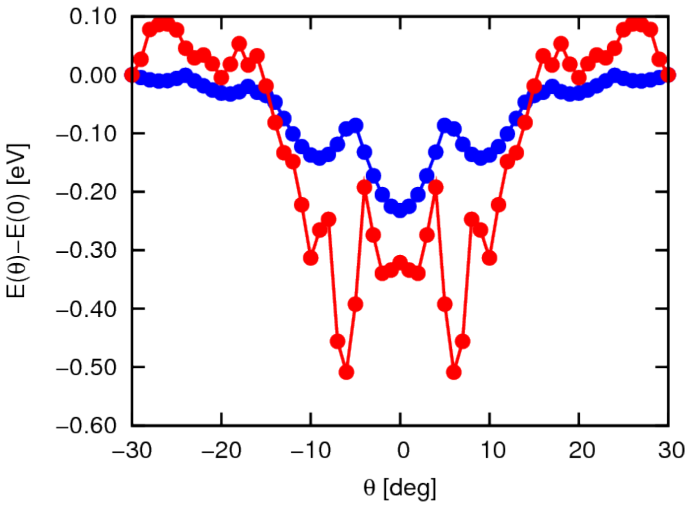


FIG. 1: Figure S1: Variation of cluster adhesion energy at $T = 0$ versus angle $\theta$ of relative orientation between cluster and substrate for the $Au_{459}$ (blue) and $Au_{1358}$ (red). The energies are obtained for fully relaxed systems. The oscillations reflect the underlying moiré between the cluster triangular (111) contact plane, and the underlying honeycomb lattice of graphene. For the $Au_{459}$ cluster the lowest energy occurs at $\theta = 0°$ with secondary minima $\pm 9°$. The energy landscape for $Au_{1358}$ is more complex, however the Novaco-McTague misalignment is already clear at $\theta = \pm 6°$ which present the lowest energies.

## Effects of constrained angular motion on cluster

We report in Fig. S2 the convergency of the measured thermophoretic force for a $Au_{459}$ cluster, with and without an applied constraint on the angular position $\theta$, deposited on a $50 \times 7\,nm^2$ graphene layer subject to a thermal gradient. The resulting $F_{th}$ are of $8.4 \pm 1.0$ pN (unconstrained $\theta$) and $8.9 \pm 0.5$ pN (constrained $\theta = 30°$), well matching within the calculated uncertainty. Note the large difference in the required time for convergency.

A more rigorous approach to the error estimate can be achieved with block-analysis. The procedure is simple: from the trajectories we collect $N$ values of the thermophoretic force $F_{th,i} = Kx_i$. We can then obtain the variance to the average $S_{avg} = \frac{1}{N}\frac{1}{N-1}\sum_{i=1}^{N} K(x_i - x_{avg})^2$. This value is an underestimate of the error, since it implies that all $N$ points of the trajectory are completely uncorrelated in time. However this is not our case since the motion of the cluster is dominated – at small timescales – by the oscillations of the dynamometric spring attached to it. To overcome this issue we group (or "block") the data. Each point $x_M$ is now the average of the force in $M$ consecutive frames of the original trajectory (or equivalently in a section of the trajectory of total time $\tau_M$). The variance to the average is then obtained by: $S^M_{avg} = \frac{1}{M}\frac{1}{M-1}\sum_{i=1}^{N/M} K(x_M - x_{avg})^2$. For uncorrelated data, this value should be constant *for all values of* $M$. In our case instead $S^M_{avg}$ does reach a plateau only for $M$ large enough so that $\tau_M$ is larger than the typical auto-correlation time of the cluster motion.

From such block analysis we measure a correlation time of $\tau \approx 3.5\,$ns for the unconstrained case, and $\tau' \approx 1\,$ns for the constrained case, see Fig. S3. The much larger $\tau$ in the former case is clearly related to the large sticking periods of the cluster when it becomes aligned with the substrate. Therefore, the much smaller $\tau'$ resulting from the angular constraint clearly reflects on the computational speed-up.

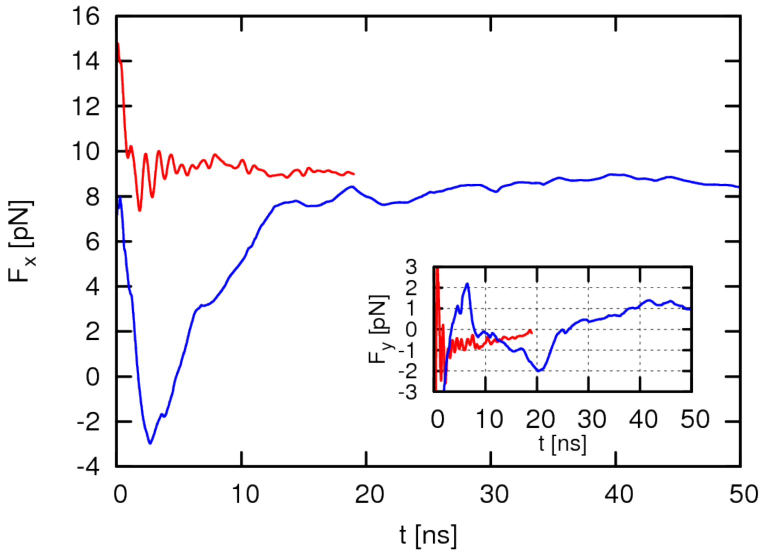


FIG. 2: Figure S2: Convergency of the average thermophoretic force in the direction parallel (perpendicular in the inset) to the thermal gradient for a $50{\times}7\,\text{nm}^2$ graphene layer clamped between $T_{hot} = 475\,$K and $T_{cold} = 325\,$K. The red lines correspond to the cluster with constrained angle $\theta = 30°$, the blue lines to the unconstrained case.

### Comments on temperature profile in ballistic and diffusive regimes

The temperature profile along graphene is the first evidence of a ballistic thermal flow. The typical profiles for purely ballistic and purely diffusive transport in the case of ideal contact resistances are depicted in Figure S4. In practical situations the observed profile lies somewhere in between the two ideal cases. We report in Fig. S5 the temperature profile for a set of graphene sheets of $L = 30$–$150\,$nm with an applied $\Delta T^0 = 150\,$K. Note that the temperature jumps decrease for larger $L$, marking the transition from ballistic to diffusive.

### Measuring the thermophoretic force from acceleration at small v

A first measure of the thermophoretic force can be obtained by studying the initial acceleration of a cluster, free to move over the graphene sheet, after the thermal gradient is switched on. However, a linear fit of the evolution of the cluster center of mass (CM) velocity, returns a value $F = mdv/dt$ that suffers of poor precision, as shown in Fig. S6 where transient acceleration is shown along with linear fit for three repeated runs. The resulting forces are $F_1 = 8.9\,$pN, $F_2 = 6.7\,$pN and $F_3 = 9.3\,$pN, which are roughly compatible with the value of $F = 8.9 \pm 0.5\,$pN obtained with the "AFM"-like setup.

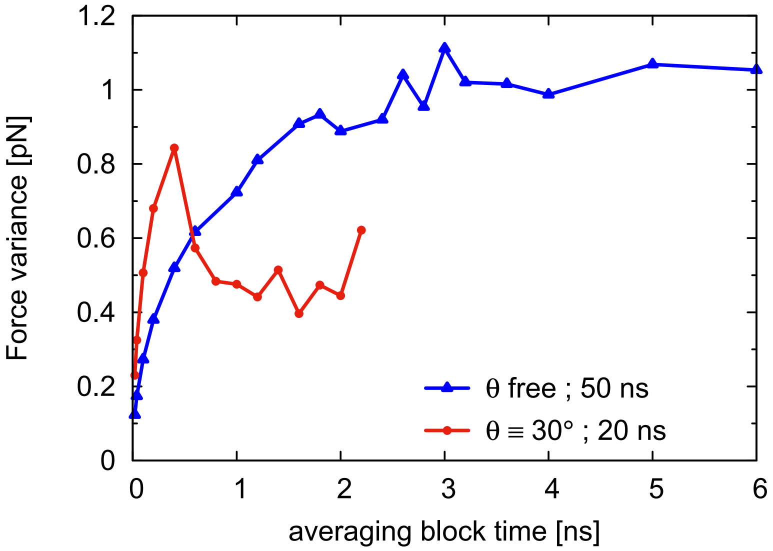


FIG. 3: Figure S3: Error estimation via block analysis for a 50 ns simulation with an unconstrained cluster angle, and a 20 ns simulation with a constrained cluster angle $\theta = 30°$. Simulation setup is otherwise identical in the two case (thermal gradient, graphene sheet size, starting configuration). The error is obtained from convergency at averaging block time $\tau_M$ larger than the autocorrelation time.

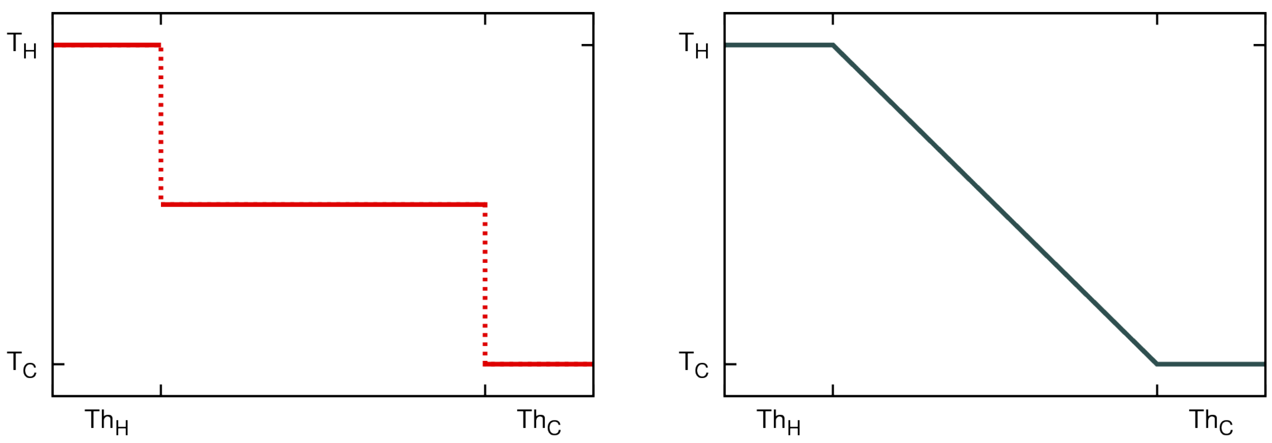


FIG. 4: Figure S4: Sketch of the temperature profile (left) in the purely ballistic regime and (right) in the purely diffusive regime for an applied temperature difference $T_H - T_C = \Delta T^0$ across the sample. Ideal thermostats are applied at Th$_H$ and Th$_C$ regions.

**Free energy contribution to thermophoresis**

The main result of our work is that the thermophoretic force arises as a scattering effect between ballistic flexural modes and the adsorbed cluster. In the scattering process some of positive physical momentum from the flexural phonon is transferred to the adsorbed cluster. However, there is also a second contribution to the thermophoretic force of purely thermodynamic origin.

A freestanding cluster in equilibrium at a temperature $T$ has a free energy $G_{Au}$. The same applies to a freestanding graphene layer, having a free energy $G_{gr}$ when in thermal equilibrium at the same temperature $T$. When the cluster is physisorbed on the graphene sheet, at equilibrium, it has a different free energy $G_{Au-C}$. The difference of free energy $\Delta G = \Delta E - T\Delta S$, where $\Delta E = E_{Au-gr} - E_{Au} - E_{gr}$ and $\Delta S = S_{Au-gr} - S_{Au} - S_{gr}$, is the adsorption free energy and will depend in general on temperature.

In a substrate endowed with a slowly varying temperature gradient, we can therefore define an adiabatic thermophoretic force as

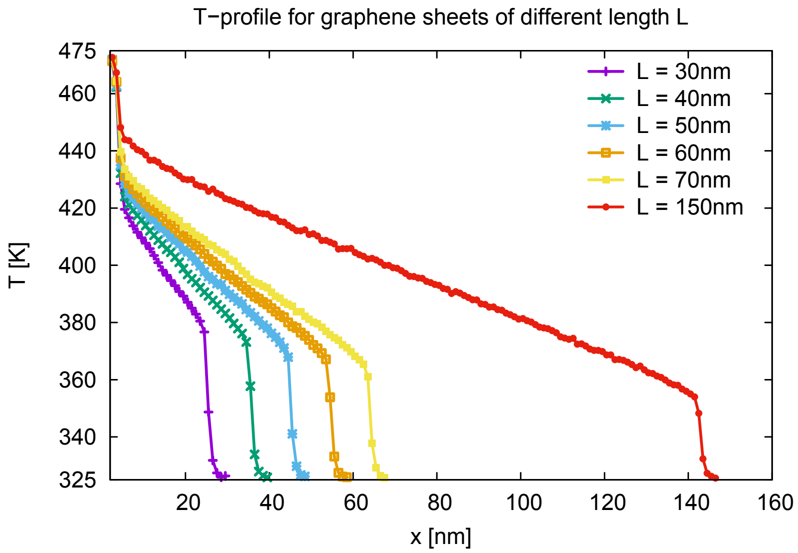


FIG. 5: Figure S5: Temperature profiles for clean graphene sheets of different length $L$ subject to a temperature difference $T_{hot} - T_{cold} = \Delta T^0 = 150\,\mathrm{K}$ between a left thermostat $T_{hot} = 475\,\mathrm{K}$ and a right thermostat $T_{cold} = 325\,\mathrm{K}$

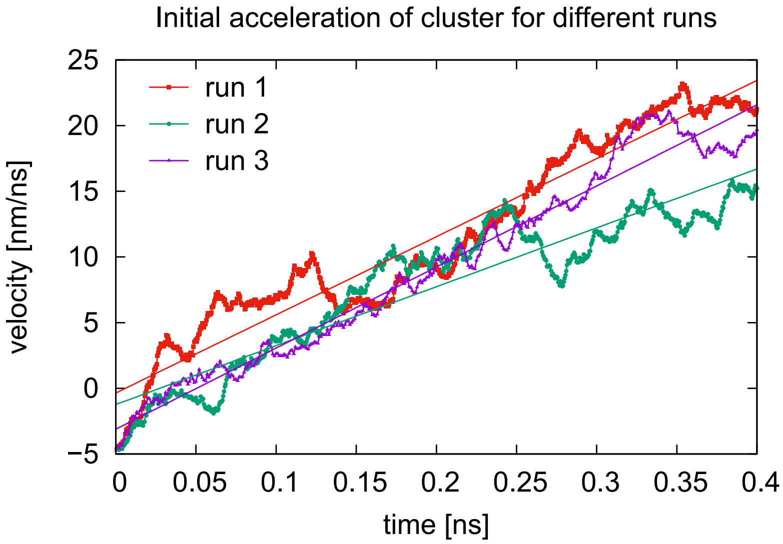


FIG. 6: Figure S6: Evolution of the velocity of the cluster CM over a $L = 50\,\mathrm{nm} \times w = 7\,\mathrm{nm}$ graphene sheet with an applied $\Delta T^0 = 150\,\mathrm{K}$. The thermal gradient is switched on at $t = 0$. Three different simulation runs are reported, different only in the initial seed of the random number generator used in the Langevin thermostats. Initial velocity at $t = 0$ fluctuates from run to run, depending on the previous thermalization stage.

$$\mathcal{F}_{th}^{ad} = -\frac{\mathrm{d}(\Delta G)}{\mathrm{d}x} = -\frac{\mathrm{d}(\Delta G)}{\mathrm{d}T}\frac{\mathrm{d}T}{\mathrm{d}x} \tag{1}$$

This force acts on the cluster in the direction where the adsorption is stronger. If, as occurs for most interfaces, the adsorption free energy deepens at lower temperatures, this thermodynamic force will push from hot to cold, as expected in thermophoresis.

We estimated such thermodynamic force contribution by evaluating $\Delta G$ as a function of $T$ by means of thermodynamic integration [5]. First, the total potential energy is expressed in terms of separated contributions from graphene (C–C), cluster (Au–Au), and mixed (Au–C) interactions:

$$U_{tot}(\lambda) = U_{gr} + U_{Au} + \lambda^4 U_{Au-gr}, \tag{2}$$

where $\lambda$ is a tunable parameter. Here $U(\lambda = 1)$ describes the physisorbed cluster on graphene, whereas $U(\lambda = 0)$ describes non-interacting cluster and graphene. The choice of $\lambda^4$ instead of a simple $\lambda$ is a convenient way to deal with divergencies in the Lennard-Jones interactions [5]. Then

$$\Delta G = \int_0^1 \mathrm{d}\lambda \left\langle \frac{\mathrm{d}U}{\mathrm{d}\lambda} \right\rangle_\lambda = \int_0^1 \mathrm{d}\lambda \left\langle 4\lambda^3 U_{Au-C} \right\rangle_\lambda, \tag{3}$$

where $\langle\cdot\rangle_\lambda$ is an equilibrium average under potential $U_{tot}(\lambda)$, to be estimated by standard MD simulations. The resulting $\Delta G(T)$ for the $Au_{459}$ cluster on a $10\times9\,\mathrm{nm}^2$ graphene sheet is $-7.81\pm0.03\,\mathrm{eV}$ at 350 K and $-7.63\pm0.03\,\mathrm{eV}$ at 450 K. These values correspond to an "adiabatic" thermophoretic force with the same direction as from simulations, i.e. from hot to cold, but a much smaller magnitude. For a typical thermal gradient of 1 K/nm the calculated force is $\mathcal{F}_{th}^{ad} = 0.3 \pm 0.1\,\mathrm{pN}$. Such thermodynamic force is very small, in fact smaller than the estimated error on the thermophoretic forces obtained in the previous sections. It can therefore be safely neglected.

## I. MEASURE OF BALLISTIC CONDUCTANCE OF GRAPHENE

The Molecular Dynamics simulations, although neglecting all quantum effects, allow us to give an estimate of the thermal conductance $\kappa A$, where $A$ is the cross-section of the graphene sheet. Since we consider sizes still in the ballistic regimes, it is more indicative to report the value of $\kappa A/L$ $[WK^{-1}m^{-2}]$, i.e. the ratio of the thermal conductance over size. For $L = 30\,\mathrm{nm}$ we obtain $\kappa A/L \sim 9\times10^9\,WK^{-1}m^{-2}$, in excellent agreement with the calculations of Mingo *et al* [6] and Muñoz *et al* [7], respectively $6\times10^9$ and $10\times10^9\,WK^{-1}m^{-2}$. The experimental values reported for suspended graphene are about one order of magnitude smaller [8]: but that is probably due to the larger sizes $L$ employed in experiments, increasingly comparable or even smaller than the MFP of some of the acoustical phonons.

[1] A. D. Novaco and J. P. McTague, Physical Review Letters **38**, 1286 (1977).
[2] D. Mandelli, A. Vanossi, N. Manini, and E. Tosatti, Phys. Rev. Lett. **114**, 108302 (2015), URL `http://link.aps.org/doi/10.1103/PhysRevLett.114.108302`.
[3] W. Luedtke and U. Landman, Physical review letters **82**, 3835 (1999).
[4] R. Guerra, U. Tartaglino, A. Vanossi, and E. Tosatti, Nature materials **9**, 634 (2010).
[5] D. Frenkel and B. Smit, Computational sciences series **1**, 1 (2002).
[6] N. Mingo and D. A. Broido, Phys. Rev. Lett. **95**, 096105 (2005), URL `https://link.aps.org/doi/10.1103/PhysRevLett.95.096105`.
[7] E. Munoz, J. Lu, and B. I. Yakobson, Nano letters **10**, 1652 (2010).
[8] E. Pop, V. Varshney, and A. K. Roy, MRS bulletin **37**, 1273 (2012).
